# Supplementary material for: Breathing Mode of a Bose-Einstein Condensate Immersed in a Fermi Sea
Source: arXiv:1911.10582 source file (2020-09-03)
Supplement: Supplementary file 1 [file supp_mat.pdf]

# Breathing mode of a BEC immersed in a Fermi sea: Supplemental Materials

Piotr T. Grochowski,[1,*] Tomasz Karpiuk,[2,†] Mirosław Brewczyk,[2,‡] and Kazimierz Rzążewski[1,§]

[1] *Center for Theoretical Physics, Polish Academy of Sciences, Aleja Lotników 32/46, 02-668 Warsaw, Poland*
[2] *Wydział Fizyki, Uniwersytet w Białymstoku, ul. K. Ciołkowskiego 1L, 15-245 Białystok, Poland*

(Dated: March 2, 2020)

## I. ENERGY OF THE UNIFORM MIXTURE

Here we present detailed schemes of calculation of the given energy spectrum – LOCV and VG.

### A. Lowest order constrained variational approach

We follow the approach from Ref. [83], however with amendments due to the repulsive character of the mixture we consider. LOCV was firstly constructed an utilized to study dense quantum fluids, e.g. liquid helium, neutron stars etc. [79]. In the context of quantum Bose-Fermi mixtures, the starting point is the Hamiltonian describing the system:

$$H = -\sum_{i=1}^{N_b} \frac{\hbar^2 \nabla_i^2}{2m_b} - \sum_{j=1}^{N_f} \frac{\hbar^2 \nabla_i^2}{2m_f} + \sum_{i,j} U_{bf}(\boldsymbol{r}_i^b - \boldsymbol{r}_j^f) + \frac{1}{2}\sum_{i,i'}^{N_b} U_{bb}(\boldsymbol{r}_i^b - \boldsymbol{r}_{i'}^b), \tag{1}$$

where $U_{bf}$ and $U_{bb}$ are zero-range pseudopotentials that are characterized by the scattering lengths, $a_{bf}$ and $a_{bb}$, consecutively. The regime that we are interested is Feshbach-tuned Bose-Fermi interaction that can be comparable to Fermi energy and therefore cannot be treated perturbatively. On the other hand, Bose-Bose interaction is small compared to other energy scales in the system and will be treated perturbatively.

The other base assumption is the Jastrow-Slater form of the trial wave function:

$$|\Psi\rangle = \prod_{i,j} f(\boldsymbol{r}_i^b - \boldsymbol{r}_j^f) \left(\frac{1}{\sqrt{V}}\right)^{N_b} |FS\rangle, \tag{2}$$

where $|FS\rangle$ is the Fermi sea of $N_f$ fermions and Jastrow function $f(\boldsymbol{r})$ describes two-body correlations between fermions and bosons and is to be variationally minimized.

The main physical assumption is that contribution of far (further than the closest one) neighbors of a given particle to instantaneous potential felt by that particle should be included only into the average field. It implies a neglect of explicit correlations between far atoms, meaning $f$ should tend to value of 1 (no distortion in the wave function) in large distances. Such a criterion is usually handled with two boundary conditions that introduce the healing length $d$, that is to be calculated self-consistently:

$$f(r = d) = 1 \tag{3}$$

$$f'(r = d) = 0, \tag{4}$$

assuming that we deal with a spherically symmetric potential.

The energy is evaluated in then so-called LOCV approximation, that takes into account only two-body term in the linked cluster expansion, giving expression in the lowest order $[O(f^2 - 1)]$:

$$\epsilon = n_b n_f \int \mathrm{d}^3\boldsymbol{r} f(\boldsymbol{r}) \left[-\frac{\nabla_{\boldsymbol{r}}^2}{2\mu} + U_{bf}(\boldsymbol{r})\right] f(\boldsymbol{r}). \tag{5}$$

---

* piotr@cft.edu.pl
† t.karpiuk@uwb.edu.pl
‡ m.brewczyk@uwb.edu.pl
§ kazik@cft.edu.pl

Before $\epsilon$ is minimized with respect to the variations in $f$, the part that comes from the average field and is not related to correlations has to be subtracted. We assume that the potential contributes only to the average field for $r > d$ and this contribution is denoted as $\lambda$. Then, the variational equation for $\epsilon$ can be written as:

$$\delta \int \mathrm{d}^3\boldsymbol{r} \left[ -f\frac{\nabla^2}{2\mu}f + fU_{bf}f - \lambda f^2 \right] = 0. \tag{6}$$

The two-body Schrödinger-like equations follows (already assuming spherical symmetry):

$$\left[ -\frac{\hbar^2}{2\mu}\frac{d^2}{dr^2} + U_{bf}(r) \right] rf(r) = \lambda rf(r). \tag{7}$$

One more constraint is needed to have a self-consistent set of equations. We need to choose healing length $d$ in such a way that on average only one particle resides within it:

$$4\pi n_f \int_0^d \mathrm{d}r r^2 f^2(r) = 1. \tag{8}$$

These equations allow to evaluate Bose-Fermi interaction energy as:

$$\epsilon_{bf} = n_b n_f \int_0^d \mathrm{d}^3\boldsymbol{r} f(\boldsymbol{r}) \left[ -\frac{\nabla^2_{\boldsymbol{r}}}{2\mu} + U_{bf}(\boldsymbol{r}) \right] f(\boldsymbol{r}) = \lambda n_b. \tag{9}$$

This equation can be rewritten as

$$\epsilon_{bf} = \lambda n_b = \frac{\hbar^2}{4\mu}(6\pi^2)^{2/3} n_f^{2/3} n_b B(\eta), \tag{10}$$

where $B(\eta)$ is a function of dimensional interaction parameter $\eta = (k_f a_{bf})^{-1}$. The details of numerical evaluation of the function $B(\eta)$ will be presented shortly.

The other part of energy spectrum is a perturbative treatment of the Bose-Bose interaction energy. Within LOCV, the correction to the mean-field energy reads:

$$\Delta\epsilon_{bb}^{LOCV} = \frac{8\pi\hbar^2}{m_b} a_{bb} n_b^2 D(\eta), \tag{11}$$

where

$$D(\eta) = n_f \int \mathrm{d}^3\boldsymbol{r} \left[ f(\boldsymbol{r}) - 1 \right]^2. \tag{12}$$

Then, the whole energy spectrum of the uniform mixture in LOCV approximation can be written as:

$$\epsilon_{LOCV} = \frac{6^{5/3}\hbar^2\pi^{4/3}}{20m_f} n_f^{5/3} + \frac{(6\pi^2)^{2/3}\hbar^2}{4\mu} n_f^{2/3} n_b B(\eta) + \frac{2\pi\hbar^2}{m_b} a_{bb} n_b^2 (1 + 4D(\eta)) \tag{13}$$

Now, we proceed to numerical evaluation of the function $B(\eta)$ and $D(\eta)$. Eq. 7 is just a usual Schrödinger type equation with a short-range pseudopotential. It yields one bound state and a continuum of scattering states. In Ref. [82] authors analyzed the bound solution, or in a language of polaron physics – the attractive branch of the energy spectrum. We are however interested in the repulsive mixture and therefore we shall investigate a lowest scattering state that satisfies boundary conditions coming from the LOCV approximation.

The effect of the short-range pseudopotential can be written as the Bethe-Peierls boundary condtion,

$$\frac{(rf)'}{rf}(r = 0) = -\frac{1}{a_{bf}}. \tag{14}$$

A scattering state, satisfying this boundary condition behaves like $rf(r) \sim \sin(kr + \delta)$, where $k$ is a wavevector connected to the energy $\lambda$ by $\lambda = \hbar^2k^2/2\mu$ and $\tan\delta/k = -a_{bf}$. Let's introduce a parameter $b$, such that $kb = \arctan ka$. Then, the solution that satisfies $f(d) = 1$ reads:

$$f(r) = \frac{d}{r}\frac{\sin k(r - b)}{\sin k(d - b)}. \tag{15}$$

With conditions for a derivative and for a normalization, a set of three equations is to be solved:

$$kb = \arctan ka_{bf} \tag{16}$$

$$4\pi n_f \int_0^d f^2(r) r^2 \mathrm{d}r = 1 \tag{17}$$

$$\frac{a_{bf}}{d} = \frac{(1/kd)\tan kd - 1}{kd \tan kd + 1}. \tag{18}$$

By introducing $k_1 = kd$ and $k_2 = ka_{bf}$ and bit of algebra, the solution fo $k_1(\eta)$ can be obtained by solving single parameter function:

$$\eta^{-3} F_1(k_1) - F_2(k_1) = 0, \tag{19}$$

where

$$F_1(k1) = \frac{1}{3\pi} k_1^2 \left[ k_1 - \sin k_1 \cos \left( k_1 - 2 \arctan \left( \frac{\tan k_1 - k_1}{k_1 \tan k_1 + 1} \right) \right) \right] \tag{20}$$

$$F_2(k_1) = \left( \frac{\tan k_1 - k_1}{k_1 \tan k_1 + 1} \right)^3 \sin^2 \left( k_1 - \arctan \left( \frac{\tan k_1 - k_1}{k_1 \tan k_1 + 1} \right) \right) \tag{21}$$

The functions $B(\eta)$ and $D(\eta)$ can then be written as:

$$B(\eta) = 2\eta^2 \left( \frac{\tan k_1(\eta) - k_1(\eta)}{k_1(\eta) \tan k_1(\eta) + 1} \right)^2 \tag{22}$$

$$D(\eta) = 1 + \frac{2}{9\pi} \eta^{-3} \left( \frac{k_1(\eta)}{k_2(\eta)} \right)^3 \left( 1 - 6 \frac{k_2(\eta) - (k_1(\eta) + k_2(\eta)) \cos k_1(\eta) + (1 - k_1(\eta) k_2(\eta)) \sin k_1(\eta)}{k_1^2(\eta) \left( \sin k_1(\eta) - k_2(\eta) \cos k_1(\eta) \right)} \right), \tag{23}$$

where

$$k_2(\eta) = \frac{\tan k_1(\eta) - k_1(\eta)}{k_1(\eta) \tan k_1(\eta) + 1}. \tag{24}$$

To compare how the result compares with another approaches, let us compare the function $B(\eta)$ with quantum Monte Carlo results from Ref. [57]. The comparison is direct, as $B(\eta)$ can be also interpreted as a repulsive polaron energy divided by the Fermi energy. In Fig. 1 the comparison is presented, showing remarkable agreement.

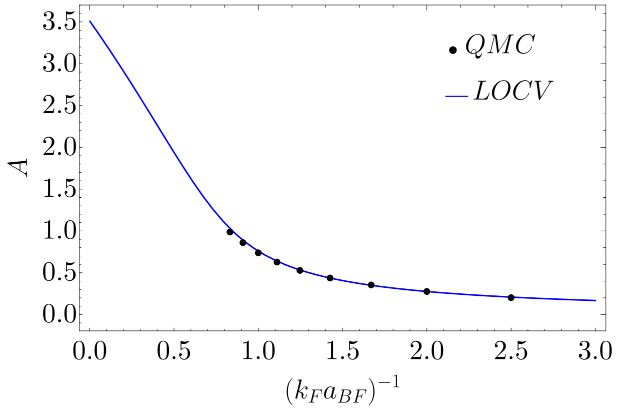


FIG. 1. Comparison of the repulsive polaron energy calculated by Quantum Monte Carlo method and in lowest order constrained variational approximation.

### B. Viverit-Giorgini perturbation scheme

Here we invoke results obtained by Ref. [76] and then generalized in Ref. [77]. The contribution to the Bose-Fermi interaction energy obtained in a frame of second-order perturbation theory leads to the following quantum correction

to the energy:

$$\epsilon_{bf}(n_b, n_f) = \epsilon_f n_b (n_f a_{bf}^3)^{2/3} A(w, \alpha) = C_{bf} a_{bf}^2 n_b n_f^{4/3} A(w, \alpha)\,, \tag{25}$$

with $C_{bf} = (6\pi^2)^{2/3}\hbar^2/2m_f$ and dimensionless parameters $w = m_b/m_f$ and $\alpha = 16\pi n_b a_{bb}/(6\pi^2)^{2/3} n_f^{2/3}$ The function $A(w, \alpha)$ is given in a form of integral:

$$A(w,\alpha) = \frac{2(1+w)}{3w}\left(\frac{6}{\pi}\right)^{2/3} \int_0^\infty \mathrm{d}k \int_{-1}^{+1} \mathrm{d}\Omega \\ \left[1 - \frac{3k^2(1+w)}{\sqrt{k^2+\alpha}} \int_0^1 \mathrm{d}q q^2 \frac{1 - \Theta(1 - \sqrt{q^2 + k^2 + 2kq\Omega})}{\sqrt{k^2+\alpha} + wk + 2qw\Omega}\right], \tag{26}$$

where $\Theta(x)$ is the step theta-function. The above formula, Eq. (25), coincides with the results of Ref. [76] for $\alpha \ll 1$, i.e. in the limit when the Fermi energy is much larger than the chemical potential of bosons.

## II. COUPLED SCHRÖDINGER-LIKE EQUATIONS

We start with a hydrodynamic (Madelung) description of bosons and fermions. Each of the species can be described in the form of a classical pseudo-wavefunction:

$$\psi = \begin{pmatrix} \psi_f \\ \psi_b \end{pmatrix} = \begin{pmatrix} \sqrt{n_f}\, e^{\mathrm{i}\frac{m_f}{\hbar}\chi_f} \\ \sqrt{n_b}\, e^{\mathrm{i}\frac{m_b}{\hbar}\chi_b} \end{pmatrix}, \tag{27}$$

where $n_j = \psi_j^\dagger \psi_j$, $j = \{b, f\}$ are one-particle densities for fermions and bosons and $\nabla\chi_j = \boldsymbol{v}_j$ are the velocity fields of the collective motion. The full system Hamiltonian is given by $H = T_{\text{tot}} + E_{\text{int}} + E_{\text{pot}}$. The total kinetic energy $T_{\text{tot}} = T + T_{\text{c}}$ consists of the intrinsic kinetic energy $T$, which in case of fermions we approximate by the Thomas-Fermi-Weizsäcker functional and in case of bosons by $\frac{\hbar^2}{2m_b}(\nabla\sqrt{n_b})^2$. The other part is the kinetic energy of the collective motion, $T_{\text{c}} = \sum_{j=b,f} \int \mathrm{d}\boldsymbol{r}\; \frac{m}{2} n_j\, \boldsymbol{v}_j^2$. The interaction and potential energies are obtained by either mean-field, LOCV or VG approaches. One can then write four Euler-Lagrange equations for the system:

$$\begin{aligned} \partial_t n_j &= -\nabla(n_j\, \boldsymbol{v}_j), \\ m\partial_t \boldsymbol{v}_j &= -\nabla\left(\frac{\delta E}{\delta n_j} + \frac{m}{2}\boldsymbol{v}_j^2\right), \end{aligned} \tag{28}$$

where the energy are evaluated with three different procedures:

$$\begin{aligned} E_{MF} &= \int \mathrm{d}^3\boldsymbol{r}\, \big(t_f(\boldsymbol{r}) + t_b(\boldsymbol{r}) + \epsilon_{bb}^0(\boldsymbol{r}) + \epsilon_{bf}^0(\boldsymbol{r}) + n_b V_b(\boldsymbol{r}) + n_f V_f(\boldsymbol{r})\big) \\ E_{LOCV} &= \int \mathrm{d}^3\boldsymbol{r}\, \big(t_f(\boldsymbol{r}) + t_b(\boldsymbol{r}) + \epsilon_{bb}^{LOCV}(\boldsymbol{r}) + \epsilon_{LHY}(\boldsymbol{r}) + \epsilon_{bf}^{LOCV}(\boldsymbol{r}) + n_b V_b(\boldsymbol{r}) + n_f V_f(\boldsymbol{r})\big) \\ E_{VG} &= \int \mathrm{d}^3\boldsymbol{r}\, \big(t_f(\boldsymbol{r}) + t_b(\boldsymbol{r}) + \epsilon_{bb}^0(\boldsymbol{r}) + \epsilon_{LHY}(\boldsymbol{r}) + \epsilon_{bf}^0(\boldsymbol{r}) + \epsilon_{bf}^{VG}(\boldsymbol{r}) + n_b V_b(\boldsymbol{r}) + n_f V_f(\boldsymbol{r})\big) \end{aligned} \tag{29}$$

The hydrodynamic equations can be however recast into the form of nonlinear Schrödinger equation by the means of inverse Madelung transformation. In the case of the mean-field it yields

$$\begin{aligned} i\hbar\partial_t\psi_f =& \Big[-\frac{\hbar^2}{2m_f}\nabla^2 + \frac{4\hbar^2}{9m_f}\frac{\nabla^2|\psi_f|}{|\psi_f|} + \frac{6^{5/3}\hbar^2\pi^{4/3}}{12m_f}|\psi_f|^{4/3} + \frac{1}{2}m_f\omega_f^2(\rho^2 + \lambda_f^2 z^2) +, \\ & \frac{2\pi\hbar^2}{\mu} a_{bf}|\psi_b|^2\Big]\psi_f, \\ i\hbar\partial_t\psi_b =& \left[-\frac{\hbar^2}{2m_b}\nabla^2 + \frac{1}{2}m_b\omega_b^2(\rho^2 + \lambda_b^2 z^2) + \frac{4\pi\hbar^2}{m_b}a_{bb}|\psi_B|^2 + \frac{2\pi\hbar^2}{\mu}a_{bf}|\psi_f|^2\right]\psi_b, \end{aligned} \tag{30}$$

In the case of LOCV:

$$i\hbar\partial_t\psi_f = \Big[ -\frac{\hbar^2}{2m_f}\nabla^2 + \frac{4\hbar^2}{9m_f}\frac{\nabla^2|\psi_f|}{|\psi_f|} + \frac{6^{5/3}\hbar^2\pi^{4/3}}{12m_f}|\psi_f|^{4/3} + \frac{1}{2}m_f\omega_f^2(\rho^2+\lambda_f^2 z^2) +, \tag{31}$$
$$\frac{2\pi\hbar^2}{\mu}a_{bf}|\psi_b|^2 R_f(\eta) - \frac{16\pi^3\hbar^2}{m_b}a_{bb}a_{bf}^3|\psi_b|^4\eta S_f(\eta)\Big]\psi_f,$$
$$i\hbar\partial_t\psi_b = \left[ -\frac{\hbar^2}{2m_b}\nabla^2 + \frac{1}{2}m_b\omega_b^2(\rho^2+\lambda_b^2 z^2) + \frac{4\pi\hbar^2}{m_b}a_{bb}|\psi_b|^2 S_b(\eta) + \frac{640\sqrt{\pi}\hbar^2}{15m_b}a_{bb}^{5/2}|\psi_b|^3 + \frac{\hbar^2}{2\mu a_{bf}^2}\frac{1}{2\eta^2}R_b(\eta)\right]\psi_b,$$

where

$$R_f(\eta) = \frac{\pi}{4}\left(2\eta B(\eta) - \eta^2 B'(\eta)\right) \tag{32}$$
$$S_f(\eta) = \eta^3 D'(\eta) \tag{33}$$
$$R_b(\eta) = B(\eta) \tag{34}$$
$$S_b(\eta) = 1 + D(\eta). \tag{35}$$

In the case of VG:

$$i\hbar\partial_t\psi_f = \Big[ -\frac{\hbar^2}{2m_f}\nabla^2 + \frac{4\hbar^2}{9m_f}\frac{\nabla^2|\psi_f|}{|\psi_f|} + \frac{6^{5/3}\hbar^2\pi^{4/3}}{12m_f}|\psi_f|^{4/3} + \frac{1}{2}m_f\omega_f^2(\rho^2+\lambda_f^2 z^2) +, \tag{36}$$
$$\frac{2\pi\hbar^2}{\mu}a_{bf}|\psi_b|^2 + \frac{2(6\pi^2)^{2/3}\hbar^2}{3m_f}a_{bf}^2|\psi_b|^2|\psi_f|^{2/3}A(\alpha) + \frac{(6\pi^2)^{2/3}\hbar^2}{2m_f}a_{bf}^2|\psi_b|^2|\psi_f|^{8/3}\frac{\partial A}{\partial\alpha}\frac{\partial\alpha}{\partial n_f}\Big]\psi_f,$$
$$i\hbar\partial_t\psi_b = \Big[ -\frac{\hbar^2}{2m_b}\nabla^2 + \frac{1}{2}m_b\omega_b^2(\rho^2+\lambda_b^2 z^2) + \frac{4\pi\hbar^2}{m_b}a_{bb}|\psi_b|^2 + \frac{640\sqrt{\pi}\hbar^2}{15m_b}a_{bb}^{5/2}|\psi_b|^3 + \frac{2\pi\hbar^2}{\mu}a_{bf}|\psi_f|^2 +,$$
$$+ \frac{(6\pi^2)^{2/3}\hbar^2}{2m_f}a_{bf}^2|\psi_f|^{8/3}A(\alpha) + \frac{(6\pi^2)^{2/3}\hbar^2}{2m_f}a_{bf}^2|\psi_b|^2|\psi_f|^{8/3}\frac{\partial A}{\partial\alpha}\frac{\partial\alpha}{\partial n_b}\Big]\psi_b,$$

## III. NUMERICAL DETAILS AND PROCEDURE

Here we present numerical details for zero temperature and nonzero temperature calculations. In numerical procedures we use the following units: length $a_{bb}$, energy $\hbar^2/(m_b a_{bb}^2)$ and time $m_b a_{bb}^2/\hbar$. To solve equations (30), (31) and (36), we use split-step methods. We use grid with dimensions $m_x = m_y = 128$ and $m_z = 1024$. Spatial steps are $\Delta x = \Delta y = \Delta z = 200\,a_{bb} = 0.6445\,\mu$m.

### A. Zero temperature

First, we look for the ground state of the mixture at zero temperature prepared in a weakly interacting state ($a_{bb} \approx 60.9a_0$ and $a_{bf} \approx 60a_0$) in an elongated trap with the aspect ratio of $\lambda = 7.6$. To do so, we solve equations (30), (31) and (36) using imaginary time technique. The time step is $\Delta t = 0.3349$ ns. Then, we propagate these equations in real time applying the excitation scheme which exactly follows the experiment. The time step for real time evolution reads $\Delta t = 3.349$ ns. After the excitation sequence, evolution still continues and we extract the condensate width according to the following formula:

$$w_b(t) = \sqrt{\int d^3r\,(x^2+y^2)\,|\psi_b|^2 \Big/ \int d^3r\,|\psi_b|^2}\,. \tag{37}$$

Finally we find the condensate frequency $\omega_b$ by fitting the expression given below:

$$w_b(t) = \alpha_b\,e^{-\gamma_b t}\sin(\omega_b\,t + \phi_b) + \beta_b + \Lambda_b\,\sin(\Omega_b\,t + \Phi_b)\,. \tag{38}$$

## B. Nonzero temperature

To prepare a thermal state we start with the ground state of the mixture initially prepared in a weakly interacting state ($a_{bb} \approx 60.9 a_0$ and $a_{bf} \approx 60 a_0$) in an elongated trap with the aspect ratio of $\lambda = 7.6$. Then we put additional energy by randomizing the wave function of bosons at each lattice location $\mathbf{r}_j$ according to the following formula:

$$\psi_b(\mathbf{r}_j) \to \psi_b^p(\mathbf{r}_j) = S_r \left[ r_1 \Re(\psi_b(\boldsymbol{r}_j)) + r_2 \Im(\psi_b(\boldsymbol{r}_j))\, i \right], \tag{39}$$

where $S_r$ is the strength of randomization, $r_1$ and $r_2$ are two random numbers chosen uniformly from $-1$ to 1 interval, $\psi_b$ is the ground state bosonic wave function and $\psi_b^p$ is the perturbed wave function. The fermionic pseudo-wave function is unperturbed at the beginning. Then, both wave functions are evolved according to the nonlinear Schrödinger equations. Depending on the case we use the version with standard meanfield terms, with VG corrections or with LOCV terms. The time evolution is conducted until we reach the thermal state. We check that by monitoring the condensate fraction. At the beginning the condensate fraction changes rapidly, then starts to saturate and finally only fluctuates around some final mean value.

In CFA the condensate fraction is extracted from the classical field by solving the eigenvalue problem for the averaged one-particle density matrix. The one particle density matrix for bosons is given by:

$$\rho_b(\boldsymbol{r}, \boldsymbol{r}', t) = \frac{1}{N_b} \psi_b^*(\boldsymbol{r}, t) \psi_b(\boldsymbol{r}', t) \,. \tag{40}$$

The eigenvalues give the occupation of modes. According to the Penrose-Onsager criterion the condensate fraction is given by the eigenvalue with the highest occupation and the condensate wave function is given by the eigenfunction corresponding to this mode. However, the one particle density matrix given by (40) is a pure state. The mixed state appears after an averaging procedure:

$$\bar{\rho}_b = \langle \rho_b(\boldsymbol{r}, \boldsymbol{r}', t) \rangle \,, \tag{41}$$

where $\langle \cdot \rangle$ may involve averaging over space, time, an ensemble or be a combination of mentioned techniques. In our case, we integrate along axial direction of the trap:

$$\bar{\rho}_b(x, y, x', y', t) = \int dz\, \psi_b^*(x, y, z, t) \psi_b(x', y', z, t) \,. \tag{42}$$

After solving the eigenvalue problem we get:

$$\bar{\rho}_b(x, y, x', y', t) = \sum_k \frac{N_b^k}{N_b} \varphi_b^{k*}(x, y, t) \varphi_b^k(x', y', t) \,,$$

where the eigenvectors $\varphi_b^k(x, y, t)$ are functions corresponding to macroscopically occupied modes:

$$\psi_b^k(x, y, t) = \sqrt{\frac{N_b^k}{N_b}}\, \varphi_b^k(x, y, t) \,,$$

and the eigenvalues $N_b^k / N_b$ give the occupations of modes. The condensate wave function averaged over axial direction is given by:

$$\psi_b^0(x, y, t) = \sqrt{\frac{N_b^0}{N_b}} \varphi_b^0(x, y, t)$$

Subtracting the column condensate density $\rho_b^0 = |\psi_b^0(x, y, t)|^2$ from the diagonal part of the one-particle density matrix one obtains the thermal cloud column density:

$$\rho_T(x, y, t) = \bar{\rho}_b(x, y, t) - |\psi_b^0(x, y, t)|^2 \,.$$

Having the thermal state we follow a similar path like at zero temperature. We apply the excitation sequence and then monitor the width of the condensate fraction. What differs is that we also can measure the width of the thermal cloud. So, we calculate both widths:

$$w_b^0(t) = \sqrt{\int d^2r\, (x^2 + y^2)\, \rho_b^0 \Big/ \int d^2r\, \rho_b^0} \,, \tag{43}$$

$$w_b^T(t) = \sqrt{\int d^2r\, (x^2 + y^2)\, \rho_T \Big/ \int d^2r\, \rho_T} \,. \tag{44}$$

Finally we find the condensate frequency $\omega_b^0$ and the thermal cloud frequency $\omega_T$ by fitting expressions given below:

$$w_b^0(t) = \alpha_b^0\, e^{-\gamma_b^0 t} \sin\left(\omega_b^0\, t + \phi_b^0\right) + \beta_b^0 + \Lambda_b^0 \sin\left(\Omega_b^0\, t + \Phi_b^0\right), \tag{45}$$

$$w_T(t) = \alpha_T\, e^{-\gamma_T t} \sin\left(\omega_T\, t + \phi_T\right) + \beta_T + \sigma_T t + \Lambda_T \sin\left(\Omega_T\, t + \Phi_T\right). \tag{46}$$

## IV. ADDITIONAL RESULTS

In Fig. 3 we present more sets of theoretical data that pertain to the experimental results from Ref. [54]. The explanation of these results is contained within the caption to that figure.

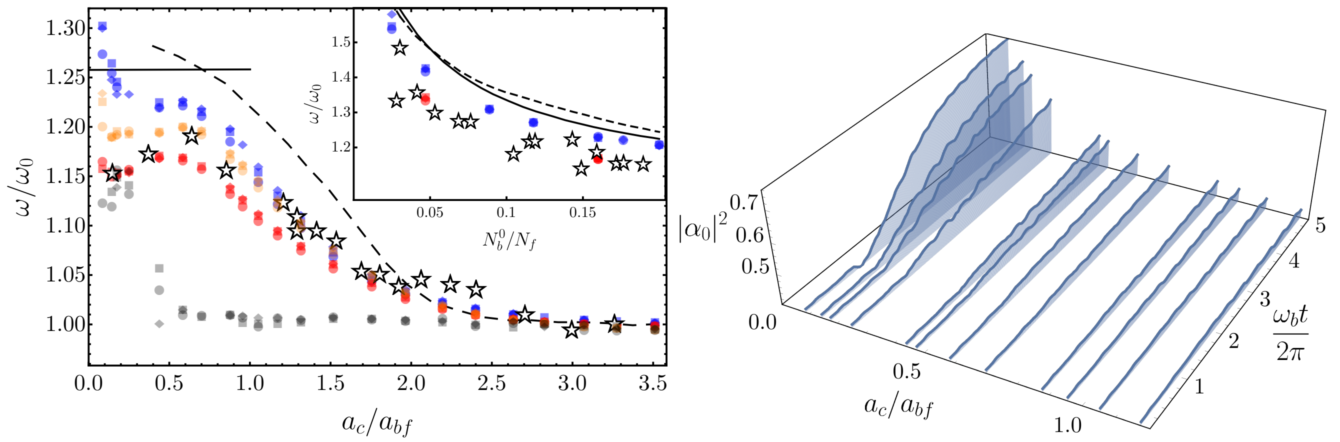


FIG. 2. (Left) The breathing mode frequency for a Bose-Einstein condensate immersed in a Fermi sea as a function of interaction parameter $a_c/a_{bf}$. The experimental data from Ref. [54] is denoted by stars. The theoretical data from Ref. [54] is indicated by black solid (full phase separation model) and black dashed (adiabatic Fermi sea model) lines. The rest of points comes from combined classical fields and pseudo-wave function model from this work. The blue color indicates zero temperature calculation, while the orange and red colors pertain to finite temperature ones. The black color signifies the oscillation frequency of the thermal cloud associated with the red markers. The circles denote bare mean field calculations, the squares – Viverit-Giorgini perturbation scheme, and the diamonds – lowest order constrained variational approach. For nonzero temperature calculation that involves temperature taken from the experiment [? ] (red markers), the initial condensed fraction of bosons is 40% and the ratio of condensed bosons to fermions is $N_b^0/N_f = 0.16$. The orange markers denote lower temperature, with the same $N_b^0/N_f = 0.16$, but with the condensed fraction being 53%. The theory from Ref. [54] clearly overestimates the experimental curve and does not reproduce nonmonotonicity for a strong interaction. So does the zero temperature calculation, however to lesser extent. The full nonzero temperature calculation grasps the experimental data both qualitatively and quantitatively. For a strong interaction, up-shift of thermal cloud's frequency is observed. (Left, inset) The breathing mode frequency as a function of number of condensed bosons to number of fermions ratio, $N_b^0/N_f$. The interaction strength is kept constant, at $a_c/a_{bf} = 0.45$. Analogously, the blue markers pertain to the zero temperature model and the red ones to the nonzero one. Again, the former overestimates the experimental data, however to the lesser extent than FPS and APS models. Accounting for a finite temperature allows to reproduce the experimental results. (Right) The fraction of condensed bosons (associated with the red markers from the left figure) as a function of time and the interaction strength. For a weak interaction it stays at the initial value, while for a strong one it increases in time and saturates at some value.

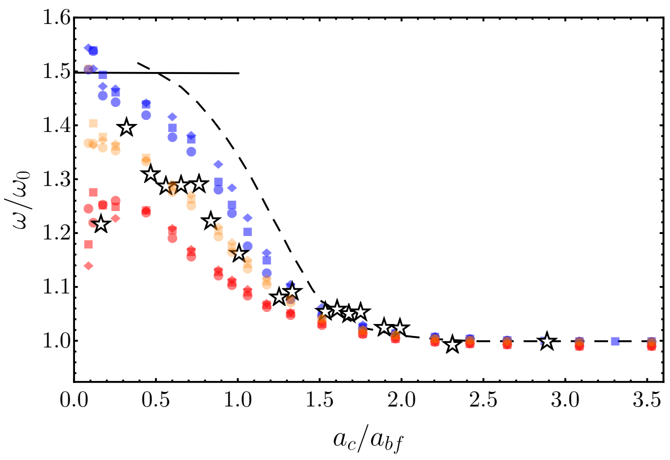


FIG. 3. (Left) The breathing mode frequency for a Bose-Einstein condensate immersed in a Fermi sea as a function of interaction parameter $a_c/a_{bf}$. The experimental data from Ref. [54] is denoted by stars. The theoretical data from Ref. [54] is indicated by black solid (full phase separation model) and black dashed (adiabatic Fermi sea model) lines. The rest of points comes from combined classical fields and pseudo-wave function model from this work. The blue color indicates zero temperature calculation, while red and orange colors pertain to finite temperature ones. The circles denote bare mean field calculations, the squares – Viverit-Giorgini perturbation scheme, and the diamonds – lowest order constrained variational approach. For nonzero temperature calculations, the initial condensed fraction of bosons vary from 20% (red markers) to 40% (orange markers). The number of condensed bosons equals 8000 and the number of fermions equals 170000. It yields the ratio of condensed bosons to fermions, $N_b^0/N_f = 0.047$. One can see that also in this case, introduction of a finite temperature reproduces the experimental data.
